# Supplementary material for: Light, Unstable Sterile Neutrinos: Phenomenology, a Search in the IceCube Experiment, and a Global Picture
Source: arXiv:2110.02351 source file (2021-10-05)
Supplement: Supplementary file 1 [file supplementary_material.pdf]

# Supplementary Material

### Illustrating tension between appearance and disappearance

Suppl. Fig. 1 and Suppl. Fig. 2 show frequentist allowed regions to separate fits to the appearance datasets and disappearance datasets at 95% confidence level, on plots of $\Delta m^2_{41}$ versus $\sin^2 2\theta_{\mu e}$. Suppl. Fig. 1 shows results for a 3+1 model, while Suppl. Fig. 2 shows results for a 3+1+decay model, separated into three lifetime decades. The disappearance datasets include IceCube. The best-fit points for each fit are indicated. In neither model is there overlap in the appearance and disappearance confidence intervals at 95%, indicating tension in the fits.

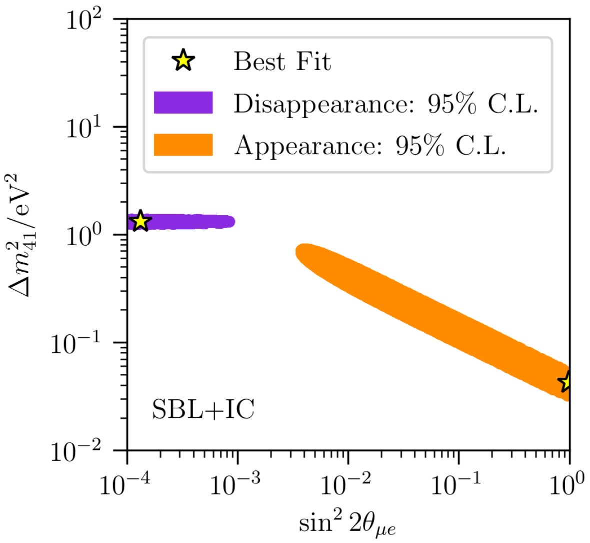


SUPPL. FIG. 1: ***Preferred regions for separate appearance and disappearance 3+1 fits.*** Frequentist 95% C.L. regions for fits to a 3+1 model, performed separately to appearance-only data and disappearance-only data, are shown. There is no overlap, indicating tension in the fits.

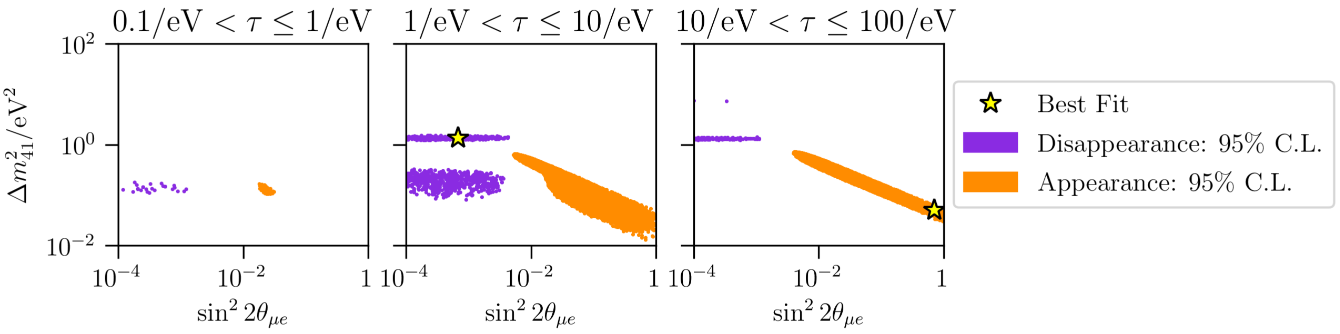


SUPPL. FIG. 2: ***Preferred regions for separate appearance and disappearance 3+1+decay fits.*** Frequentist 95% C.L. allowed regions for fits to a 3+1+decay model, performed separately to appearance-only data and disappearance-only data, are shown. There is no overlap, indicating tension in the fits.

**Preferred regions of 3+1+decay**

Suppl. Fig. 3 and Suppl. Fig. 4 show the global-fit result for a 3+1+decay model at 95% C.L. as a function of the three relevant parameters: lifetime ($\tau$), heavy neutrino mass ($m_4$), and appearance amplitude ($\sin^2 2\theta_{\mu e}$). Suppl. Fig. 3 shows the result for Short-Baseline only (left) and IceCube incorporated (right). Suppl. Fig. 4 shows the result including IceCube, where the preference for each parameter point is indicated by the marker size.

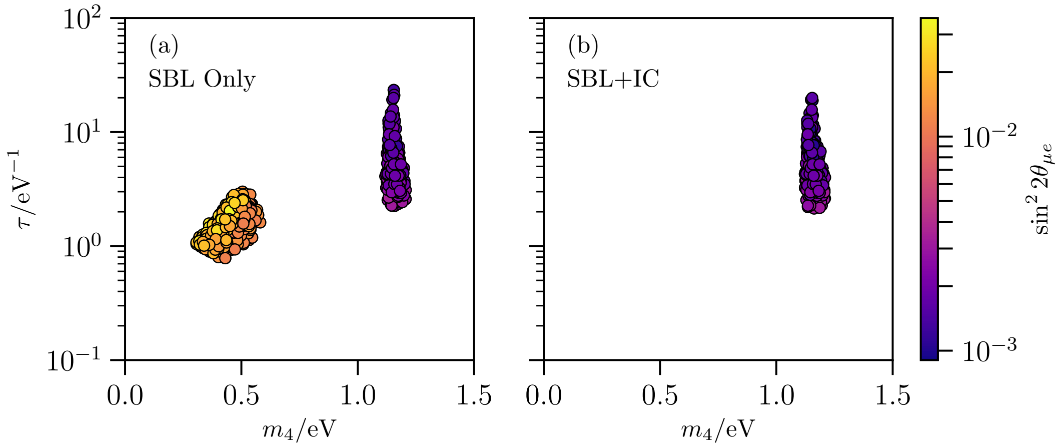


SUPPL. FIG. 3: ***3+1+Decay model allowed regions at 90% C.L.*** The left panel shows the allowed regions when considering only the SBL dataset, while the right panel shows them with IceCube included. In both panels, the horizontal axis shows the new mass state mass, $m_4$, the vertical axis its lifetime, $\tau$, and the color scale the appearance amplitude. When considering only the SBL data two populations exist: one with large mixings and small masses ($\sin^2 2\theta_{\mu e} \sim 10^{-2}$ and $m_4 \sim 0.5$ eV) and another with smaller mixing and larger masses ($\sin^2 2\theta_{\mu e} \sim 10^{-3}$ and $m_4 \sim 1.25$ eV). When including IceCube the large mass population is removed. For $\tau = 1$ eV$^{-1}$, $c\tau = 0.2$ $\mu m$.

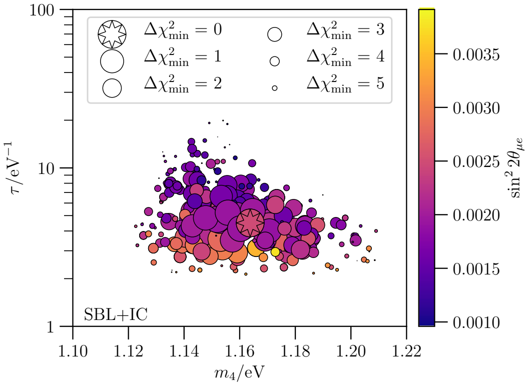


SUPPL. FIG. 4: ***3+1+Decay model allowed regions using the SBL and IceCube data at 95% C.L. shown with parameter point preference.*** In this figure the markers show the preference for a particular point, the horizontal axis shows the new mass state mass, $m_4$, the vertical axis its lifetime, $\tau$, and the color scale the mixing amplitude. The best-fit point is shown as the largest marker with the star symbol imprinted. Points with decreasing preference, with respect to the best-fit point, are drawn with smaller markers. For $\tau = 1$ eV$^{-1}$, $c\tau = 0.2$ $\mu m$.

## List of experiments included

The data sets used in this work include neutrino and antineutrino sets; they are are:

- **Muon-to-electron neutrino appearance ($\nu_\mu \to \nu_e$)**: MiniBooNE (BNB) [1], MiniBooNE (NuMI) [2], NOMAD [3], LSND [4], and KARMEN [5].

- **Muon-neutrino disappearance ($\nu_\mu \to \nu_\mu$)**: SciBooNE/MiniBooNE [6], CCFR [7], CDHS [8], MINOS [9], and IceCube [10].

- **Electron-neutrino disappearance ($\nu_e \to \nu_e$)**: KARMEN/LSND cross section [11], Bugey [12], NEOS [13], DANSS [14], SAGE [15], GALLEX [16], and PROSPECT [17].

## Table of $\chi^2$

Suppl. Tbl. I reports the $\chi^2$ obtained for the two different models considered in this work. For each model, we report the best-fit $\chi^2$ for the short-baseline dataset only and this set with IceCube included as different columns. We also report the $\chi^2$ obtained when separating the data into appearance and disappearance experiments in order to evaluate the parameter goodness of fit.

| Fit type<br>Dataset | $3\nu$ (Null)<br>SBL | $3\nu$ (Null)<br>SBL+IC | 3+1<br>SBL | 3+1<br>SBL+IC | 3+1+Decay<br>SBL | 3+1+Decay<br>SBL+IC |
|---|---|---|---|---|---|---|
| Best fit | | | | | | |
| $\chi^2$/dof | 492.7 / 509 | 672.5 / 718 | 458.4 / 506 | 640.8 / 715 | 449.9 / 505 | 631.84 / 714 |
| p-value | 0.69 | 0.89 | 0.94 | 0.98 | 0.96 | 0.99 |
| Null vs. Sterile | | | | | | |
| $\Delta\chi^2/\Delta$dof | | | 34.3 / 3 | 31.7 / 3 | 42.8 / 4 | 40.7 / 4 |
| p-value: | | | 1.7E-07 | 6.0E-07 | 1.2E-8 | 3.1E-8 |
| $N\sigma$ | | | 5.1 | 4.9 | 5.6 | 5.4 |
| 3+1 vs. 3+1+decay | | | | | | |
| $\Delta\chi^2/\Delta$dof | | | | | 8.5 / 1 | 9.0 / 1 |
| p-value: | | | | | 0.0036 | 0.0027 |
| $N\sigma$ | | | | | 2.7 | 2.8 |
| PG Test | | | | | | |
| $(\chi^2/\text{dof})_{\text{app}}$ | | | 77.3 / 2 | 77.3 / 2 | 77.4 / 3 | 77.4 / 3 |
| $(\chi^2/\text{dof})_{\text{dis}}$ | | | 355.8 / 3 | 535.5 / 3 | 355.8 / 4 | 535.4 / 4 |
| $(\chi^2/\text{dof})_{\text{glob}}$ | | | 458.4 / 3 | 640.8 / 3 | 449.9 / 4 | 631.8 / 4 |
| $(\chi^2/\text{dof})_{\text{PG}}$ | | | 25.2 / 2 | 28.0 / 2 | 16.7 / 3 | 19.0 / 3 |
| $p$-value | | | 3.4E-6 | 8.1E-7 | 8.0E-4 | 2.7E-4 |
| $N\sigma$ | | | 4.5 | 4.8 | 3.2 | 3.5 |

SUPPL. TABLE I: ***Summary of $\chi^2$ obtained in this global fit for different models, datasets and splits.*** Each column corresponds to a particular combination of model ($3\nu$, 3+1, or 3+1+decay) and dataset (SBL or SBL plus IceCube, SBL+IC). The first section gives the best-fit $\chi^2$, degrees of freedom (dof), and p-value. The second section compares a given sterile model (3+1 or 3+1+decay) and the three-neutrino model via the $\chi^2$ difference for best-fit parameters for a fixed dataset. The third section contains the comparison between the 3+1 and 3+1+decay models, both with and without IceCube data. Finally, the fourth section reports the p-value for the parameter goodness of fit test for the 3+1 and 3+1+decay models, both with and without IceCube data.

### Oscillation probabilities at best-fit parameter points

Suppl. Fig. 5 shows the oscillation probabilities at the best-fit parameter points for the 3+1 and 3+1+decay models. This figure is meant to illustrate and provide intuition on the difference between these two models and help understand why one is preferred over the other in our fits. Thus, we compare the oscillation probabilities relevant to three categories of experiments included in our fits: (left) short-baseline reactor measurements, (center) MiniBooNE, and (right) long-baseline accelerator measurements, like MINOS. In each plot, we show the oscillation probability averaged over each energy bin, with a binning chosen to reflect that used in the relevant experiment or experiment category. At the longest baselines, the 3+1 oscillations vary so rapidly with energy that the energy resolution of the detector prohibits resolving individual oscillation peaks. This makes the long-baseline muon-neutrino disappearance analysis a normalization only search, which are known to be less sensitive than shape analyses. The best-fit 3+1+decay parameters predicts a normalization slightly closer to the null hypothesis than the best-fit 3+1 parameters do. At the smallest baselines and lowest energies of reactor experiments, the oscillations are damped and only noticeable at larger energies where the reactor neutrino statistics are smaller. Finally, for MiniBooNE's energies and baseline, the shape predicted by the two models remains similar, but the normalization is increased in the decay scenario.

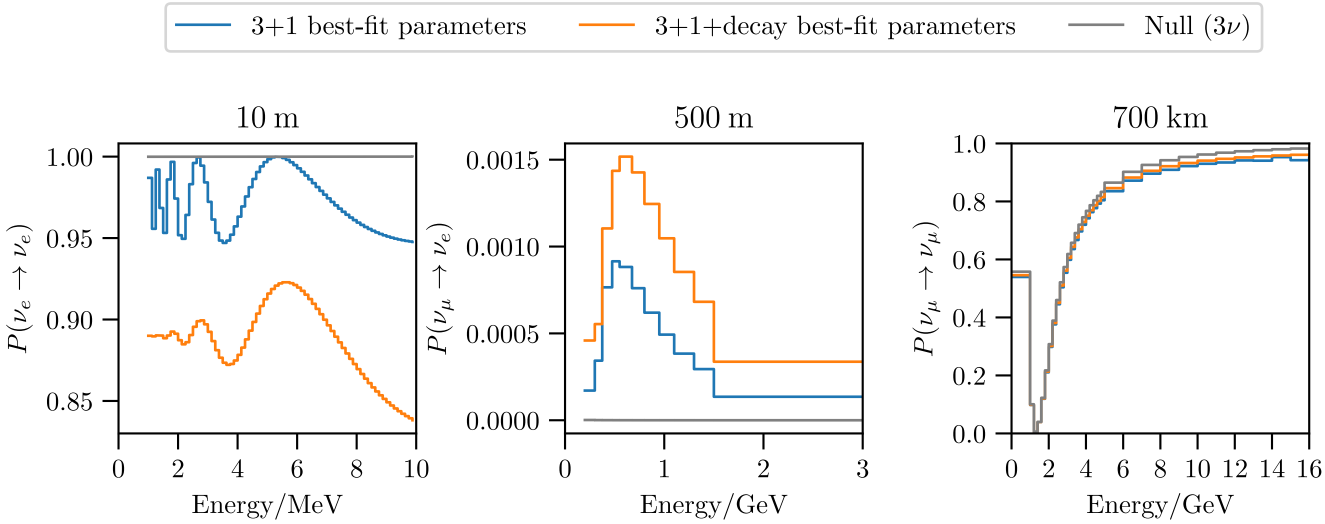


SUPPL. FIG. 5: ***Illustration of transition probabilities.*** In these figures, blue indicates the 3+1 model at best-fit parameters, orange indicates the corresponding point in the 3+1+decay model, and grey indicates the null hypothesis (three neutrinos). In each panel, probabilities plotted are the average over each bin in energy, where the binning is chosen to reflect the experimental binning. The left panel shows the electron-neutrino survival probability in the energy range relevant for reactor experiments at a ten meter baseline. The center panel shows the muon-neutrino to electron-neutrino appearance probability for the energy and baseline scales relevant for the MiniBooNE measurement. Finally, the right panel shows the muon-neutrino survival probability for the energy range of long-baseline neutrino experiments that probe the atmospheric oscillation scale, like MINOS. In this panel, the 3+1 oscillations occur too rapidly to be resolved.

[1] A. A. Aguilar-Arevalo et al. (MiniBooNE), Phys. Rev. Lett. **121**, 221801 (2018), 1805.12028.
[2] P. Adamson et al. (MiniBooNE, MINOS), Phys. Rev. Lett. **102**, 211801 (2009), 0809.2447.
[3] P. Astier et al. (NOMAD), Phys. Lett. **B570**, 19 (2003), hep-ex/0306037.
[4] C. Athanassopoulos et al. (LSND), Phys. Rev. Lett. **81**, 1774 (1998), nucl-ex/9709006.
[5] B. Armbruster et al. (KARMEN), Phys. Rev. **D65**, 112001 (2002), hep-ex/0203021.
[6] K. B. M. Mahn et al. (SciBooNE, MiniBooNE), Phys. Rev. **D85**, 032007 (2012), 1106.5685.
[7] I. E. Stockdale et al., Phys. Rev. Lett. **52**, 1384 (1984).
[8] F. Dydak et al., Phys. Lett. **134B**, 281 (1984).
[9] P. Adamson et al. (MINOS), Phys. Rev. Lett. **117**, 151803 (2016), 1607.01176.
[10] M. G. Aartsen et al. (IceCube), Phys. Rev. Lett. **117**, 071801 (2016), 1605.01990.
[11] J. M. Conrad and M. H. Shaevitz, Phys. Rev. **D85**, 013017 (2012), 1106.5552.

[12] Y. Declais et al., Nucl. Phys. **B434**, 503 (1995).
[13] Y. J. Ko et al. (NEOS), Phys. Rev. Lett. **118**, 121802 (2017), 1610.05134.
[14] I. Alekseev et al. (DANSS), Phys. Lett. **B787**, 56 (2018), 1804.04046.
[15] J. N. Abdurashitov et al. (SAGE), Phys. Rev. **C80**, 015807 (2009), 0901.2200.
[16] F. Kaether, W. Hampel, G. Heusser, J. Kiko, and T. Kirsten, Phys. Lett. **B685**, 47 (2010), 1001.2731.
[17] J. Ashenfelter et al. (PROSPECT), Phys. Rev. Lett. **121**, 251802 (2018), 1806.02784.
